# Supplementary material for: Thermally-Enhanced Fr\"ohlich Coupling in SnSe
Source: arXiv:1905.09174 source file (2019-05-22)
Supplement: Supplementary file 1 [file SM.pdf]

# Supplemental Materials for "Thermally Enhanced Polar Electron-Phonon Coupling in SnSe"

Fabio Caruso, Maria Troppenz, Santiago Rigamonti, and Claudia Draxl

*Institut für Physik and IRIS Adlershof,*

*Humboldt-Universität zu Berlin, Berlin, Germany*

## SUPPLEMENTARY NOTE 1: COMPUTATIONAL DETAILS

Band-structure calculations are based on Kohn-Sham density-functional theory (DFT) [1, 2], as implemented in `Quantum Espresso` [3]. We use the Perdew-Burke-Ernzerhof (PBE) version of the generalized-gradient approximation for the exchange-correlation functional [4]. Core electrons are accounted for via Troullier-Martin norm-conserving pseudo-potentials [5], whereas Sn $5s/5p$ and Se $4s/4p$ electronic orbitals are treated explicitly and expanded in a plane-wave basis set with a 816 eV kinetic energy cutoff. Bloch wave-vectors are sampled on a $4\times8\times8$ Mockhost-Pack grid. Phonons and Born-effective charges are obtained from density-functional perturbation theory [6] on a $2\times4\times4$ mesh of $\mathbf{q}$-points. Electron energies, phonons frequencies, and electron-phonon matrix elements are interpolated using maximally-localized Wannier functions [7] from the `Wannier90` library [8]. The electron-phonon self-energy $\Sigma$ is evaluated within the Fan-Migdal approximation as implemented in the `EPW` code [9], whereas the (static) Debye-Waller term is approximately accounted for by imposing conservation of the number of particles through $\mathrm{Re}\Sigma_{n\mathbf{k}}(\omega = \varepsilon_\mathrm{F}) = 0$, where $\varepsilon_\mathrm{F}$ is the Fermi energy. Integrals over momentum are performed on a random $\mathbf{q}$-point mesh consisting of 88942 points sampled according to a Cauchy distribution. Temperature is accounted for via the Fermi-Dirac and Bose-Einstein occupation factors.

Calculations of the electrical conductivity have been performed within the full-potential all-electron density-functional theory code **`exciting`** [10], using the PBE exchange-correlation functional [4] and the linearized Boltzmann equation in the relaxation-time approximation [11]. Muffin-tin radii of 2.0 for both Sn and Se are employed, and the basis set size is determined by the dimensionless parameter $R_\mathrm{MT}|\mathbf{G}+\mathbf{k}|_\mathrm{max} = 10$. For the density and the potential, a plane-wave cutoff $G_\mathrm{max}$ of 20 ${a_0}^{-1}$ is applied. We use a homogeneous $4 \times 12 \times 12$ $\mathbf{k}$-point mesh for the ground-state calculation, and a dense mesh of $20 \times 60 \times 60$ $\mathbf{k}$-points, leading to 10571 $\mathbf{k}$-points in the irreducible Brillouin zone, to obtain reliable tensor components of the conductivity.

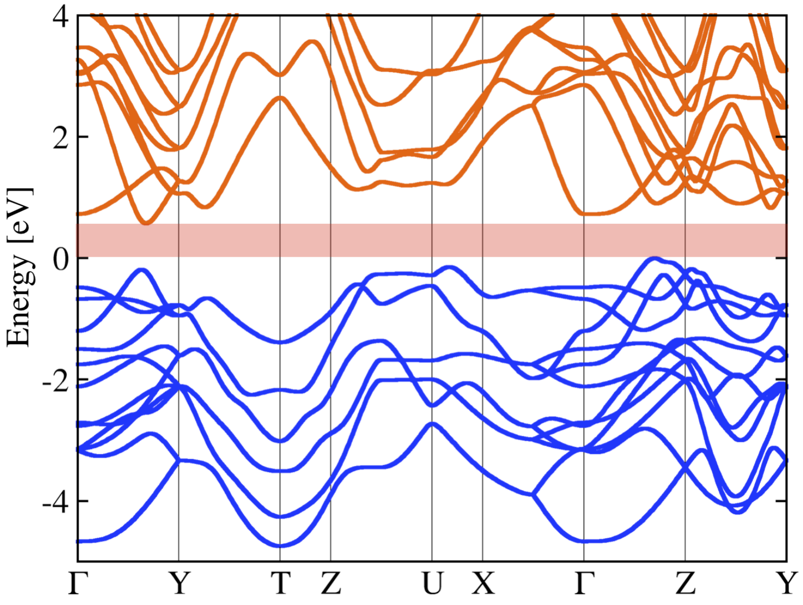


Supplementary Fig. 1. Electron band structure as obtained from DFT with the PBE exchange correlation functional. The fundamental gap between the occupied (blue) and empty (orange) manifold is shaded.

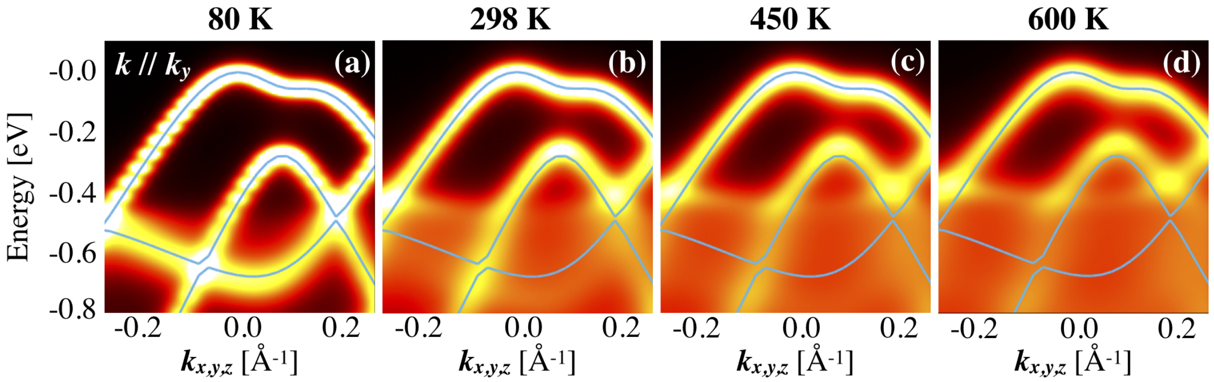


Supplementary Fig. 2. Temperature dependence of the angle-resolved spectral function for the valence bands for crystal momenta along the $\mathbf{k}_y$ direction in the Brillouin zone at 80, 297, 450, and 600 K. The DFT bands (light blue) are superimposed for comparison.

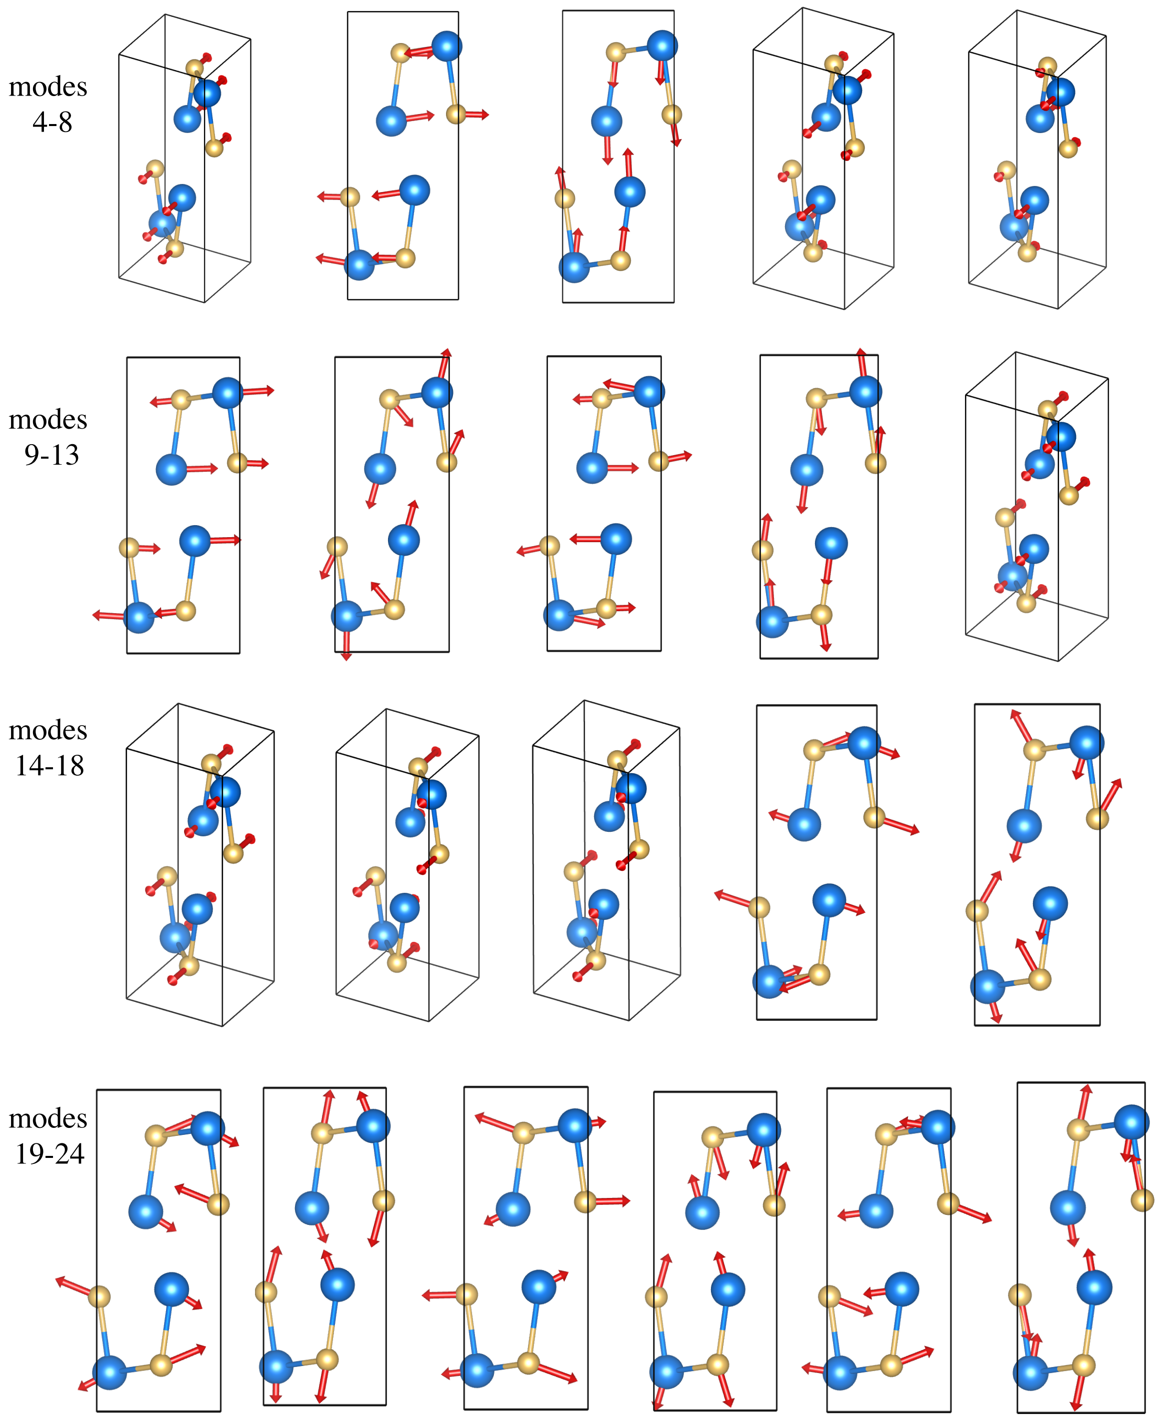


Supplementary Fig. 3. Schematic representation of the atomic displacement due to the 21 optical phonon modes of SnSe, as obtained from DFPT through the diagonalization of the dynamical matrix at $\mathbf{q} = (0, 0, 0.005)$ Å$^{-1}$.

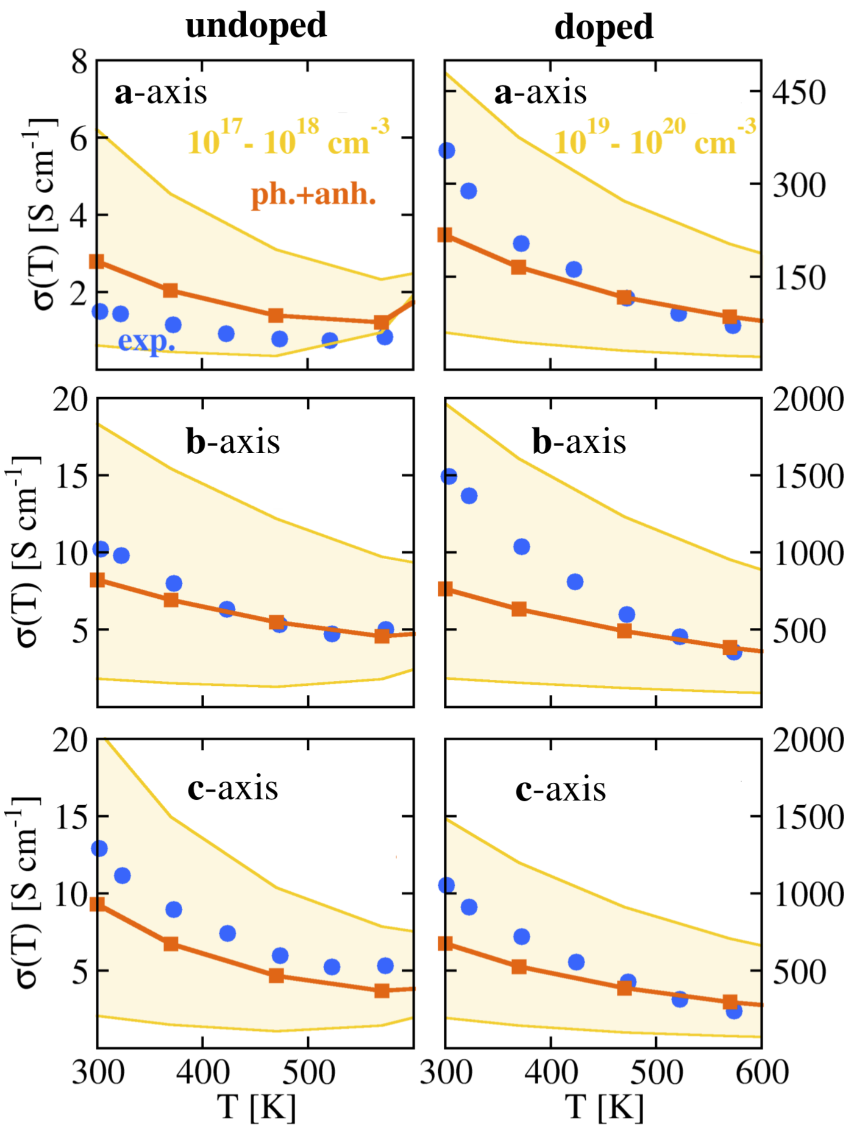


Supplementary Fig. 4. Temperature dependence of electrical conductivity along the **a** [(a) and (b)], **b** [(c) and (d)], **c** [(e) and (f)] crystal axes when accounting for both lattice anharmonicity and electron-phonon coupling (orange square) compared to experiment (blue circles). The left column shows results for undoped SnSe, whereas in the right column we consider a $p$-type doping concentration of $4 \cdot 10^{19}\,\mathrm{cm}^{-3}$. The shaded area indicates the values span by the electrical conductivity for carrier concentrations in the range $10^{17} - 10^{18}\,\mathrm{cm}^{-3}$ (left) and $10^{19} - 10^{20}\,\mathrm{cm}^{-3}$ (right). Experimental data are taken from Ref. [12].

[1] P. Hohenberg and W. Kohn, Phys. Rev. **136**, B864 (1964).

[2] W. Kohn and L. J. Sham, Phys. Rev. **140**, A1133 (1965).

[3] P. Giannozzi *et al.*, J. Phys.: Condens. Matter **21**, 395502 (2009).

[4] J. P. Perdew, K. Burke, and M. Ernzerhof, Phys. Rev. Lett. **77**, 3865 (1996).

[5] N. Troullier and J. L. Martins, Phys. Rev. B **43**, 1993 (1991).

[6] S. Baroni, S. de Gironcoli, A. Dal Corso, and P. Giannozzi, Rev. Mod. Phys. **73**, 515 (2001).

[7] N. Marzari, A. A. Mostofi, J. R. Yates, I. Souza, and D. Vanderbilt, Rev. Mod. Phys. **84**, 1419 (2012).

[8] A. A. Mostofi, J. R. Yates, Y.-S. Lee, I. Souza, D. Vanderbilt, and N. Marzari, Comput. Phys. Commun. **178**, 685 (2008).

[9] S. Poncé, E. Margine, C. Verdi, and F. Giustino, Comput. Phys. Commun. **209**, 116 (2016).

[10] A. Gulans, S. Kontur, C. Meisenbichler, D. Nabok, P. Pavone, S. Rigamonti, S. Sagmeister, U. Werner, and C. Draxl, Journal of Physics: Condensed Matter **26**, 363202 (2014).

[11] T. J. Scheidemantel, C. Ambrosch-Draxl, T. Thonhauser, J. V. Badding, and J. O. Sofo, Phys. Rev. B **68**, 125210 (2003).

[12] L.-D. Zhao, G. Tan, S. Hao, J. He, Y. Pei, H. Chi, H. Wang, S. Gong, H. Xu, V. P. Dravid, C. Uher, G. J. Snyder, C. Wolverton, and M. G. Kanatzidis, Science (2015).
